# Supplementary material for: Bridging Personalization and Control in Scientific Personalized Search
Source: arXiv:2411.02790 source file (2025-04-30)
Supplement: Supplementary file 1 [file supp-materials.tex]

\newpage
\section{Appendix}
\subsection{Experimental Setup}
\subsubsection{Datasets} We use a public benchmark for personalized search \cite{bassani2022person}. Given that realistic user interactions are not commonly released publicly due to privacy concerns, \citet{bassani2022person} construct a benchmark for personalized search from paper authorship and citation network data. Here, they treat authors of scientific papers as a user $u$ performing a search, and $u$'s most recent published paper $d_q$ is used to generate a query $q$ and the list of relevant documents for $q$. The title for $d_q$ is treated as a query, and all of the papers cited in $d_q$ are treated as relevant to $q$. The users previously authored papers are treated as their historical interactions $D_u$ for personalization. %\hamed{Please make sure appendix is allowed!}

\subsubsection{Baselines}
\label{sec-baselines-supp}
We consider a range of standard personalized and non-personalized retrieval approaches spanning sparse retrieval, dense retrieval, cross-encoders, and ensemble methods. 

Our non-personalized approaches span: \ul{BM25}: A standard unsupervised sparse retrieval baseline based on term overlap between query and document, with strong generalization performance across tasks and domains \cite{robertson2009bm25}. \ul{Contriver}: A BERT-base bi-encoder model pre-trained for zero-shot retrieval with weakly supervised query-document pairs \cite{izacard2022unsupervised}. \ul{MPNet-1B}: A strong Sentence-Bert bi-encoder model initialized with MPNet-base \cite{song2020mpnet} and trained on 1 billion supervised query-document pairs aggregated from numerous domains \cite{reimers2019sentencebert}. \ul{MPNet-CQA}: A model identical to MPNet-1B, trained on 250 million question-answer pairs mined from community QA datasets. Prior work also notes this to be valuble training data for dense retrievers \cite{menon22defensedual}. \ul{CrossEnc}: A cross-encoder trained on the same data as \ctrlce while ignoring the users historical interactions, $D_u$. CrossEnc is initialized with MPNet-base \cite{song2020mpnet}, and query-document score is produced by passing the \texttt{CLS} representation through a MLP. CrossEnc represents the closest approach to \ctrlce given that it represents a non-personalized cross-encoder.

Our personalized approaches span, ensemble methods using prior personalized dense retrieval models and prior personalized cross-encoder models: \ul{\texttt{rf}(BM25, QA)}: This represents a rank-fusion based approach which learns a weighted combination of scores produced by BM25 and a Query Attention (QA) based user modeling approach. Importantly, QA is a key component of effective personalization in prior work on personalized search, \cite[HRNN-QA]{ge2018rnnqa}, \cite[ZAM]{ai2019zam}, and \cite[EDAM]{jiang2020qagoogle}. QA scores candidate documents based on their dot product similarity to weighted average of user documents. The weights for user documents are computed as dot-product attentions between query and document representations from MPNet-1B. \ul{\texttt{rf}(BM25, QA, MPNet-1B)}: This adds dense retrieval scores from MPNet-1B to the \texttt{rf}(BM25, QA) ensemble. \ul{CrossEnc$_{RA}$}: This represents a cross-encoder personalized with retrieval-augmentation \cite{salemi2023lamp}. It inputs, query, candidate, and the top-1 document most similar to the query from $D_u$. This approach follows the state of the art personalized cross-encoder model for product search \cite[CoPPS]{dai2023contrastivecross}, however given the longer length of documents in our datasets compared to products we leverage retrieval augmentation to reduce input sequence lengths. We use the MPNet-CQA model for retrieving the top-1 document. % Finally, note that while we compare to several reasonable baselines, we primarily aim to demonstrate that \ctrlce results in strong performance (Section \ref{sec-edps-expresults}, \ref{sec-edps-ablations}) while remaining controllable (Section \ref{sec-edps-inteval}) rather than establish SOTA performance.

\subsubsection{Implementation Details}
\label{sec-implementation-supp}
In implementing \ctrlce, we initialize $\texttt{Enc}_{\text{CE}}$ with MPNet-base (HF model: mpnet-base) \cite{song2020mpnet} and we initialize $\texttt{Enc}_{\text{Mem}}$ with MPNet-CQA (HF model: multi-qa-mpnet-base-cos-v1) for both \ctrlceit and \ctrlcecv. 
We formulate $g_{\text{Mix}}$ as a MLP with 1-hidden layer of 386 dimensions and use a $\texttt{tanh}$ non-linearity. In \ctrlcecv, we use MPNet-CQA to embed both profile items and profile concepts. Further, in \ctrlcecv for constructing concept-based user profiles for a concept inventory $\mathcal{K}$ we use a collection of computer science concepts for Comp Sci and an inventory of Wikipedia categories for Physics, Pol Sci, and Psych. Computer science concepts are extracted using the unsupervised method of \citet{king2020forecite} from a corpus of 2.1 million computer science and biomedical papers in the S2ORC corpus \cite{lo2020s2orc}. Further we use a profile size $P$ of size $0.5\cdot N_u$ to ensure that $\mathcal{P}_u$ remains more succinct than $D_u$. For both \ctrlcecv and \ctrlceit we use up to 300 historical documents per user (i.e.\ $N_u \leq 300$) sampling documents at random for users with $>300$ documents. We also train all the proposed models on up to 270k queries for all the datasets to keep training time reasonable. We use $M=4$ negative documents per positive selected from irrelevant documents in the first stage BM25 based ranking after position 20 of the ranked list to prevent false negatives. In our two-stage training (Section \ref{sec-edps-memce-training}) we perform 1 epoch over our training set for each stage and save the best model based on the MRR over a dev-set of 1000 queries. In training $g_{\text{Mix}}$ with our calibrated softmax objective we set $y_0=0.1$ and $y_0=0.2$ for \ctrlcecv and \ctrlceit respectively. This value was tuned between $\{0.1, 0.2, 0.3\}$ and set based on the MRR over a dev-set of 1000 queries. For first stage ranking we use BM25 as a first stage ranker and re-rank $K=200$ documents per query.
\begin{figure*}[t]
    \centering
    \subfloat[\centering \ctrlceit in Comp Sci]{{\includegraphics[width=4.3cm]{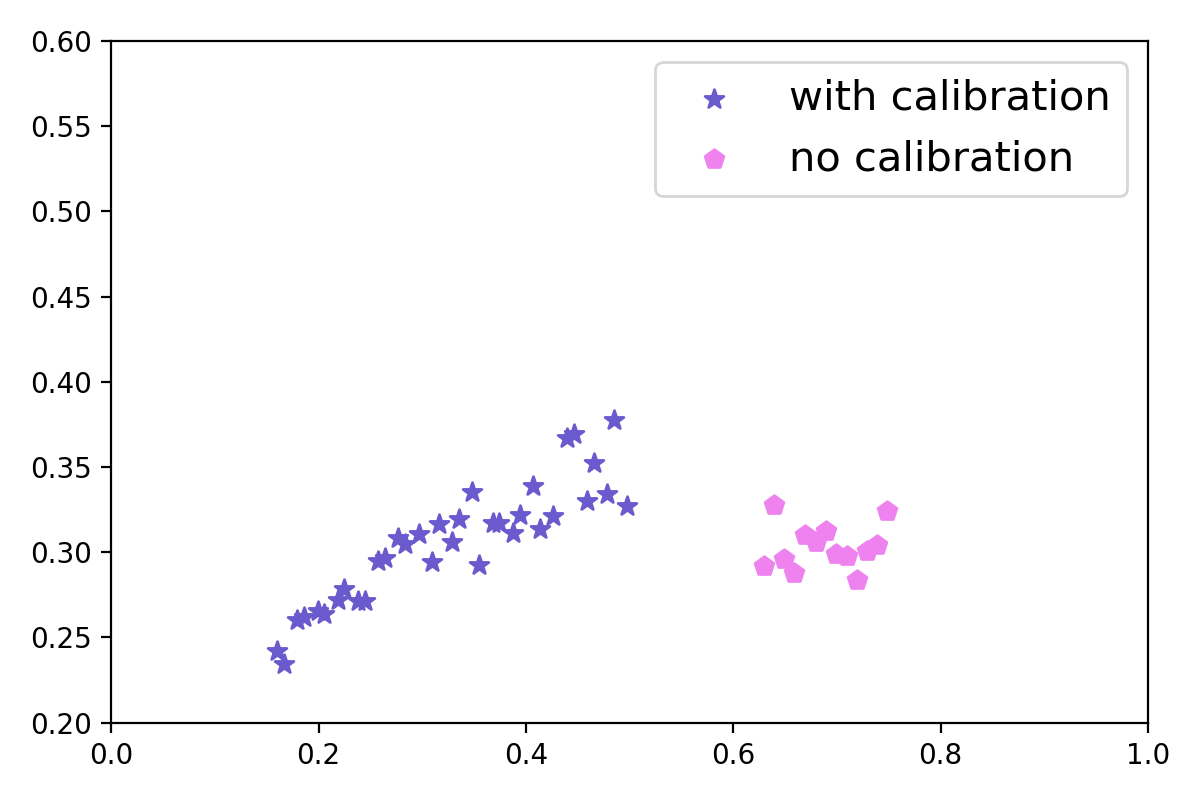}}}%
    ~
    \subfloat[\centering \ctrlceit in Physics]{{\includegraphics[width=4.3cm]{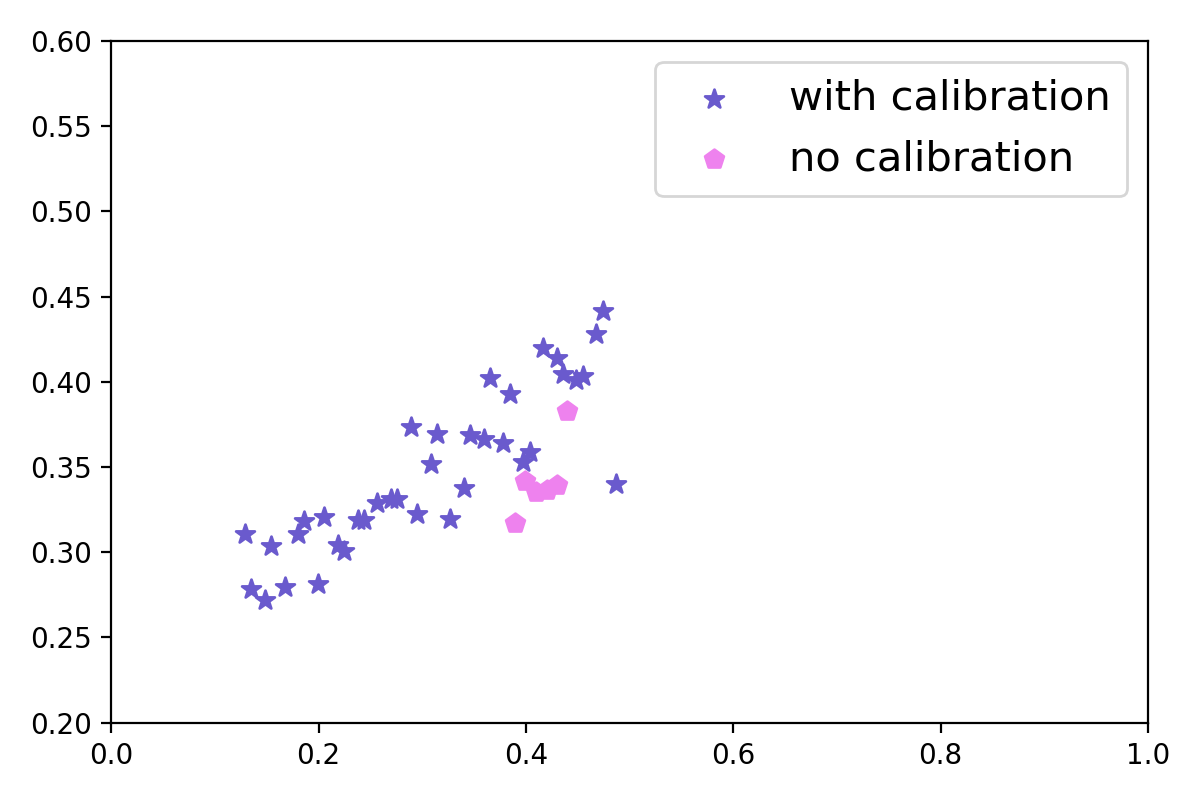}}}%
    ~
    \subfloat[\centering \ctrlceit in Pol Sci]{{\includegraphics[width=4.3cm]{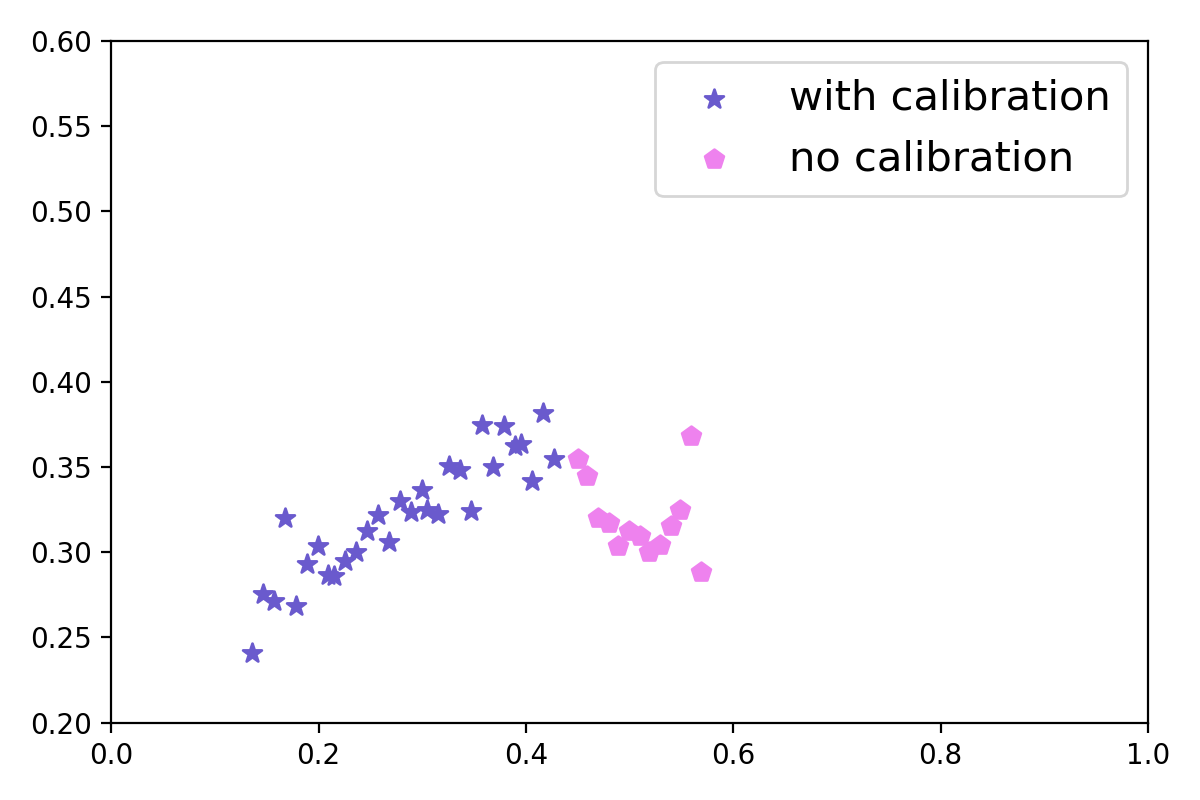}}}%
    ~
    \subfloat[\centering \ctrlceit in Psych]{{\includegraphics[width=4.3cm]{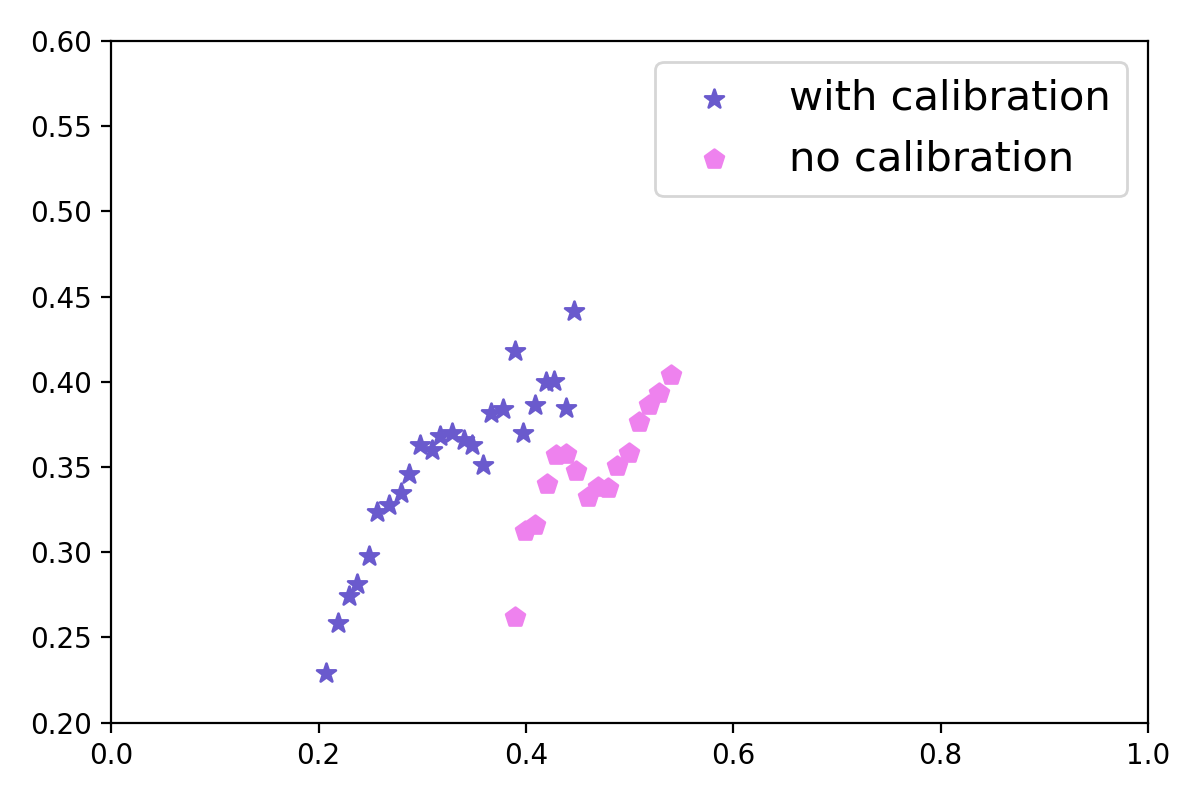}}}%
    \caption{Scores produced by the mixing model $g_{\text{Mix}}$ used to combine $f_{\text{CE}}$ and $f_{\text{Mem}}$ as $f=w\cdot f_{\text{CE}} + (1-w)\cdot f_{\text{Mem}}$ plotted against the NDCG@10 metric for the rankings produced by $f_{\text{CE}}$. \ctrlceit (blue) is compared against the respective models trained without a calibrated objective (pink). Our calibrated objective ensures that $g_{\text{Mix}}$ remains proportional to $f_{\text{CE}}$ performance. Section \ref{sec-edps-calibeval} discusses these results further.}%
    \label{fig-edps-person-calibration-it}%
\end{figure*}
